# Supplementary material for: Computing Floquet Hamiltonians with Symmetries
Source: arXiv:2007.06112 ancillary file (2020-07-23)

In[12]:= **r7 = PadeApproximant[Log[1 + z], {z, 0, {7, 7}}]**

$$\text{Out[12]= } \frac{z + 3z^2 + \frac{535z^3}{156} + \frac{145z^4}{78} + \frac{1377z^5}{2860} + \frac{223z^6}{4290} + \frac{11z^7}{7280}}{1 + \frac{7z}{2} + \frac{63z^2}{13} + \frac{175z^3}{52} + \frac{175z^4}{143} + \frac{63z^5}{286} + \frac{7z^6}{429} + \frac{z^7}{3432}}$$

In[13]:= **ExpandAll[240 240 Numerator[p7]]**

Out[13]= 240 240 p7

In[14]:= **ExpandAll[240 240 Denominator[p7]]**

Out[14]= 240 240

In[15]:= **2 ^ 5**

Out[15]= 32

In[16]:= **Exp[i Pi / 32]**

Out[16]=  $e^{\frac{i\pi}{32}}$

In[17]:= **N[Abs[1 - e <sup>$\frac{i\pi}{32}$</sup> ]]**

Out[17]= 0.0981353

In[18]:= **f = ReplaceAll[r7, z → -x]**

$$\text{Out[18]= } \frac{-x + 3x^2 - \frac{535x^3}{156} + \frac{145x^4}{78} - \frac{1377x^5}{2860} + \frac{223x^6}{4290} - \frac{11x^7}{7280}}{1 - \frac{7x}{2} + \frac{63x^2}{13} - \frac{175x^3}{52} + \frac{175x^4}{143} - \frac{63x^5}{286} + \frac{7x^6}{429} - \frac{x^7}{3432}}$$

In[19]:= **g = Log[1 - x]**

Out[19]= Log[1 - x]

In[25]:= `Plot[f - g, {x, -0.1, 0.1}, PlotPoints -> 200, MaxRecursion -> 12]`

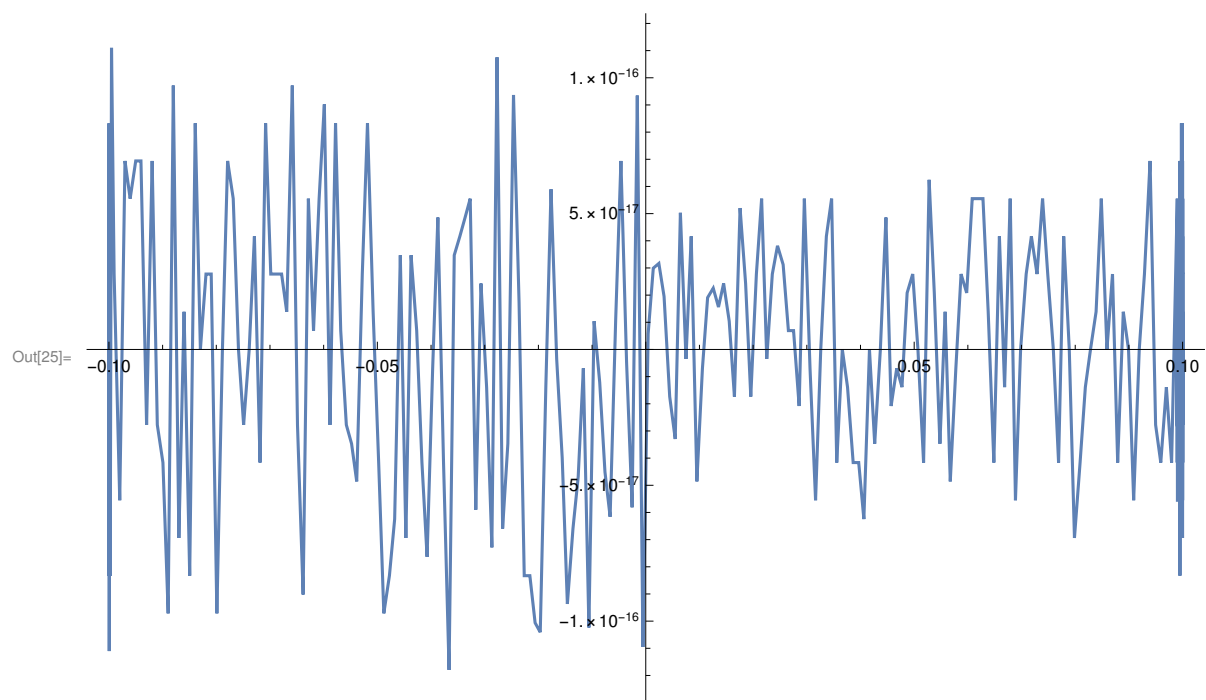

Supplement: Supplementary file 1 [file PadeError.pdf]
